# Supplementary material for: On the Frequency Bias of Generative Models
Source: arXiv:2111.02447 source file (2021-11-03)
Supplement: Supplementary file 1 [file sec_abstract.tex]

\begin{abstract}
In this \textbf{supplementary document}, 
we first provide implementation details on the testbeds for the generator and the discriminator in ~\secref{sec:testbeds}.
In~\secref{sec:generator} and~\secref{sec:discriminator} we include additional analyses for the generator and discriminator, respectively.
\secref{sec:gans} comprises additional results for full GAN training.
Lastly, we provide details on the datasets in ~\secref{sec:datasets}.
The \textbf{supplementary video} shows additional visualizations for the experiment in Fig. 1 of the main paper. 
\end{abstract}
